# Supplementary material for: GaussianMotion: End-to-End Learning of Animatable Gaussian Avatars with Pose Guidance from Text
Source: arXiv:2502.11642 source file (2025-02-17)
Supplement: Supplementary file 2 [file supple.tex]

\clearpage
\setcounter{page}{1}
\setcounter{section}{0}
\setcounter{table}{0}
\setcounter{figure}{0}
\maketitlesupplementary

%\section{Supplementary: Overview}
%\label{sec:overview}
%In this supplementary material, we present additional experiments.
% We first provide details of our training process and network architectures in {\it Training Detail} and {\it Network Architecture Detail} section, 
% and those of derivation of transformation matrices in {\it Derivation Detail} section. 
% Lastly, we provide the additional results and the challenging cases of our method in {\it Additional Results} section. 

% \vspace{10cm}

\section{Training Details}

\noindent {\bf Implementation detail}
%Implementation detail
The trainable parameters in our model include the 3D Gaussian points and the blend weight network $f_{\theta_r}$, which predicts the residual blend weights for rigid transformations (refer to \eqref{eq:blend_weight} for the definition of blend weights).
The 3D Gaussian points are initialized with $N = 70k$ points, randomly sampled from the SMPL mesh surface in the canonical space.
The blend weight network $f_{\theta_r}$ is implemented as a multilayer perceptron (MLP) with four hidden layers, each consisting of 128 dimensions. It takes $\mathbf{x}_c \in \mathbb{R}^3$ (without positional encoding) as input and outputs a 24-dimensional vector, corresponding to the 24 joints defined in the SMPL model.
%\todo{texture network 얘기도}

We train our model for a total of $20k$ iterations, which requires approximately 90 minutes on a single NVIDIA RTX 3090 GPU. 
The ADAM optimizer is used with $\beta_1 = 0.9$ and $\beta_2 = 0.999$. 
The learning rate for the 3D Gaussian points follows the configuration suggested in the original implementation by \cite{qian20233dgs}, while the learning rate for the blend weight network $f_{\theta_r}$ is set to $1 \times 10^{-4}$.  
Additionally, an exponential learning rate scheduler is applied to progressively decrease the learning rate by a factor of 0.1 for the blend weight network.

We utilized Stable Diffusion V1.5~\cite{rombach2022high} as the base diffusion model for score distillation and employed the pretrained pose-conditioned ControlNet~\cite{zhang2023adding} available from the library of state-of-the-art pretrained diffusion models ({\small  \url{https://huggingface.co/lllyasviel/control_v11p_sd15_openpose}}).

In Adaptive Score Distillation, we set $\tau = 450$ and $s = 22.5$, representing the timestep threshold for denoising score integration and the guidance scale for CFG sampling, respectively.
To further enhance the output quality of our method, we employ the annealed distillation time schedule~\cite{wang2024prolificdreamer}, which reduces the maximum timestep to 500 starting from the 1000th iteration. For the full definition of the score matching difference, please refer to \eqref{eq:ads}.

In the total training objective, we set $\lambda_{\text{scale}} = 1000$ and $\lambda_{\text{skinning}} = 1$ across all experiments. The skinning loss $\mathcal{L}_{\text{skinning}}$ is defined as:

\begin{equation}
\mathcal{L}_{\text {skinning}}=\frac{1}{|\mathcal{P}|} \sum_{p \in \mathcal{P}} \left\|\mathbf{w}(\mathbf{x}_c)-\mathbf{w}^{\mathbf{S}}(\mathbf{x}_c)\right\|_2^2,
\label{eq:skinning}
\end{equation}
where $\mathcal{P}$ denotes the set of all Gaussians defined in the canonical space.

%그외 모든 파라미터 명시 
\noindent {\bf Rendering Detail in the Training} 
To facilitate convergence, we render the front or back views of the canonical pose with a probability of 0.2, while random poses are rendered with a probability of 0.8 at each iteration.
For random poses, the pose parameters are sampled from a normal distribution $\mathcal{N}(0, 1)$, scaled by 0.3, and the viewing angle is randomly selected from an azimuth range of $[-180^\circ, 180^\circ]$. Additionally, we crop $256 \times 256$ patches from the full-body rendered images to focus on finer details in local regions of the generated output.

\noindent {\bf Adaptive Density Control} 3DGS adaptively adjusts the resolution of Gaussian points using Adaptive Density Control (ADC). This mechanism periodically adds or removes points based on predefined criteria, such as position gradients, scaling factors, or opacity values.

Starting with an initial set of $70k$ sparse points on the SMPL mesh, we perform ADC every 100 iterations. Following the original 3DGS strategy, Gaussians are cloned and split when the average magnitude of view-space position gradients surpasses a threshold, which we set to 0.02 in our method. 
%Additionally, points are cloned if the mean distance to the $k=5$ nearest Gaussian points exceeds 0.02, to prevent sparsity. 

Additionally, points are cloned if the mean distance to the $k = 5$ nearest Gaussian points exceeds 0.02. This ensures that sparsely distributed Gaussian points are filled in, leading to a more dense representation.
%Pruning is applied when the scaling factor is greater than 0.1, or if the 3D Gaussian points deviate by more than 0.1 in distance from the nearest SMPL vertex.
Pruning is applied when the scaling factor exceeds 0.1 or when a 3D Gaussian point is located more than 0.1 away from its nearest SMPL vertex. This ensures the removal of floating points that stray too far from the underlying SMPL structure, maintaining a more compact representation.

\noindent {\bf View prompting} The Janus problem, where multiple heads appear in the output, is a common issue in text-to-3D tasks. It occurs because the diffusion model generates outputs from a canonical viewpoint, influenced by the training data distribution, specifically the canonical pose in the human domain. 

%We mitigate this issue through view prompting, augmenting the input prompt with view-dependent descriptors like ’front view,’ ’back view,’ and ’side view,’ while interpolating the text embeddings based on the azimuth sampled during training. 

We mitigate this issue through view prompting by augmenting the input prompt with view-dependent descriptors such as 'front view', 'back view', and 'side view'. The text embeddings are encoded from each augmented prompt and interpolated based on the azimuth angle sampled during training.

%\section{Additional Experiments}
%limitation 
%more ablation study 
%residual blend weight? 

% \begin{figure*}[t]
% \centering
% %\def\arraystretch{0.2}
% \begin{tabular}{@{}c}
% \includegraphics[width=0.9\linewidth]{Figures/quali_supple_2.pdf} \\
% \end{tabular}
% \caption{{\bf Qualitative comparison of 3D human models.} We evaluate our approach against recent state-of-the-art baselines using different prompts. 
% %viewpoints of 0 and 60 degrees,
% }
% \label{fig:quali_supple}
% \end{figure*}

\section{Derivation Detail}
\label{sec:derivation_detail}

The position coordinate $\mathbf{x}_c$ of Gaussian splats are transformed into the observation space using the transformation matrix $\mathbf{B}$ by ~\eqref{eq:transform} in the main paper. 
As described in the main paper,  $\mathbf{B}$ can be computed from the given body pose $\mathbf{p}$. The body pose is defined as $\mathbf{p} =(\mathbf{J}, \boldsymbol{\theta})$, where $\mathbf{J} = \{\mathbf{j}_i\}$ consists of $B$ joint locations, and $\boldsymbol{\theta} = \{\boldsymbol{\omega}_i\}$ defines relative rotation of each body part with respect to its parent joint using the axis-angle representation. $\mathbf{B}_b$ of $b$-th skeleton part is computed as follows,
%transformation matrix of $k$-th skeleton part that maps the bone's coordinates from the target to the canonical space.

\begin{equation}
\mathbf{B}_b=  A_b(\mathbf{J}, \boldsymbol{\theta}^{\text{obs}}) A_b(\mathbf{J}, \boldsymbol{\theta}^\text{c}) ^{-1},
\end{equation}

\begin{equation}
A_b(\mathbf{J}, \boldsymbol{\theta})=\prod_{i \in P(b)}\left[\begin{array}{cc}
R\left(\boldsymbol{\omega}_i\right) & \mathbf{j}_i \\
0 & 1
\end{array}\right],
\end{equation}

\noindent where $R(\boldsymbol{\omega}_i) \in\mathbb{R}^{3\times3}$ is the rotation matrix converted from $\boldsymbol{\omega}_i$ using the Rodrigues formula, $\mathbf{j}_i$ is the coordinate of $i$-th joint, and $P(b)$ is the ordered set of parent joints of $b$-th joint.

%user study text 목록
\section{Test Set Prompts}
We use the following 30 prompts for our test set, which is employed in both quantitative evaluation and user studies. These prompts are sampled from the list provided by HumanGaussian~\cite{liu2024humangaussian} to ensure fair comparisons.

\begin{framed}
    \noindent 1. A boy with a beanie wearing a hoodie and joggers. \\
    2. A body builder wearing a tanktop. \\
    3. A Viking. \\
    4. A Black woman wearing sunglasses, a white t-shirt and jeans. \\
    5. A Texas ranger. \\
    6. A Black man wearing a green t-shirt. \\
    7. A Black woman wearing a hoodie. \\
    8. A woman wearing ski clothes. \\
    9. A Black man wearing a red baseball cap. \\
    10. A Black woman dressed in gym clothes. \\
    11. A woman wearing a short jean skirt, a cropped top, and a white sneaker. \\
    12. A fairy. \\
    13. A knight. \\
    14. A vampire hunter. \\    
    15. A revenant. \\    
    16. A vigilante. \\    
    17. A warlock. \\    
    18. An alchemist. \\    
    19. An alien. \\    
    20. A man with a black fedora and a denim jacket. \\
    21. A man with a brown fedora and a denim jacket. \\
    22. A woman with a pink beanie. \\
    23. A man with a buzz cut wearing a red t-shirt. \\
    24. A woman with a side shave wearing a black t-shirt. \\
\end{framed}
\begin{framed}
    \noindent 
    25. A man with messy hair wearing a gray sweater. \\
    26. A person with a curly beard and a black hoodie. \\
    27. A bounty hunter. \\
    28. A cyborg. \\
    29. A demon slayer. \\
    30. A dryad.
\end{framed}

\section{Additional Comparison}

%We provide additional qualitative comparisons with state-of-the-art text-to-3D human methods~\cite{kolotouros2024dreamhuman,liao2024tada,huang2024humannorm, liu2024humangaussian} in \figref{fig:quali_supple}. 
We present direct one-to-one comparisons against the most recent state-of-the-art models, HumanNorm~\cite{huang2024humannorm} and HumanGaussian~\cite{liu2024humangaussian}, in \figref{fig:quali_supple_humannorm} and \figref{fig:quali_supple_humangaussian}, respectively.
%As shown in the figures, our method consistently produces fine-grained details with clean, natural animations, while HumanGaussian suffers from severe artifacts during pose changes, and HumanNorm's overall full-body quality remains overly simplistic.
As demonstrated in the figures, HumanGaussian suffers from severe artifacts during pose changes, which arise from mapping errors between the Gaussian points and the mesh surface during zero-shot articulation.
On the other hand, HumanNorm struggles to capture complex body structures and textures, resulting in overly simplistic and unrealistic reconstructions. This limitation is evident in the lack of detailed representation for hands and clothing.
In contrast, our method consistently produces fine-grained details with clean and natural animations, effectively capturing intricate features.

\begin{figure*}[t]
\centering
\begin{tabular}{@{}c}
\includegraphics[width=0.9\linewidth]{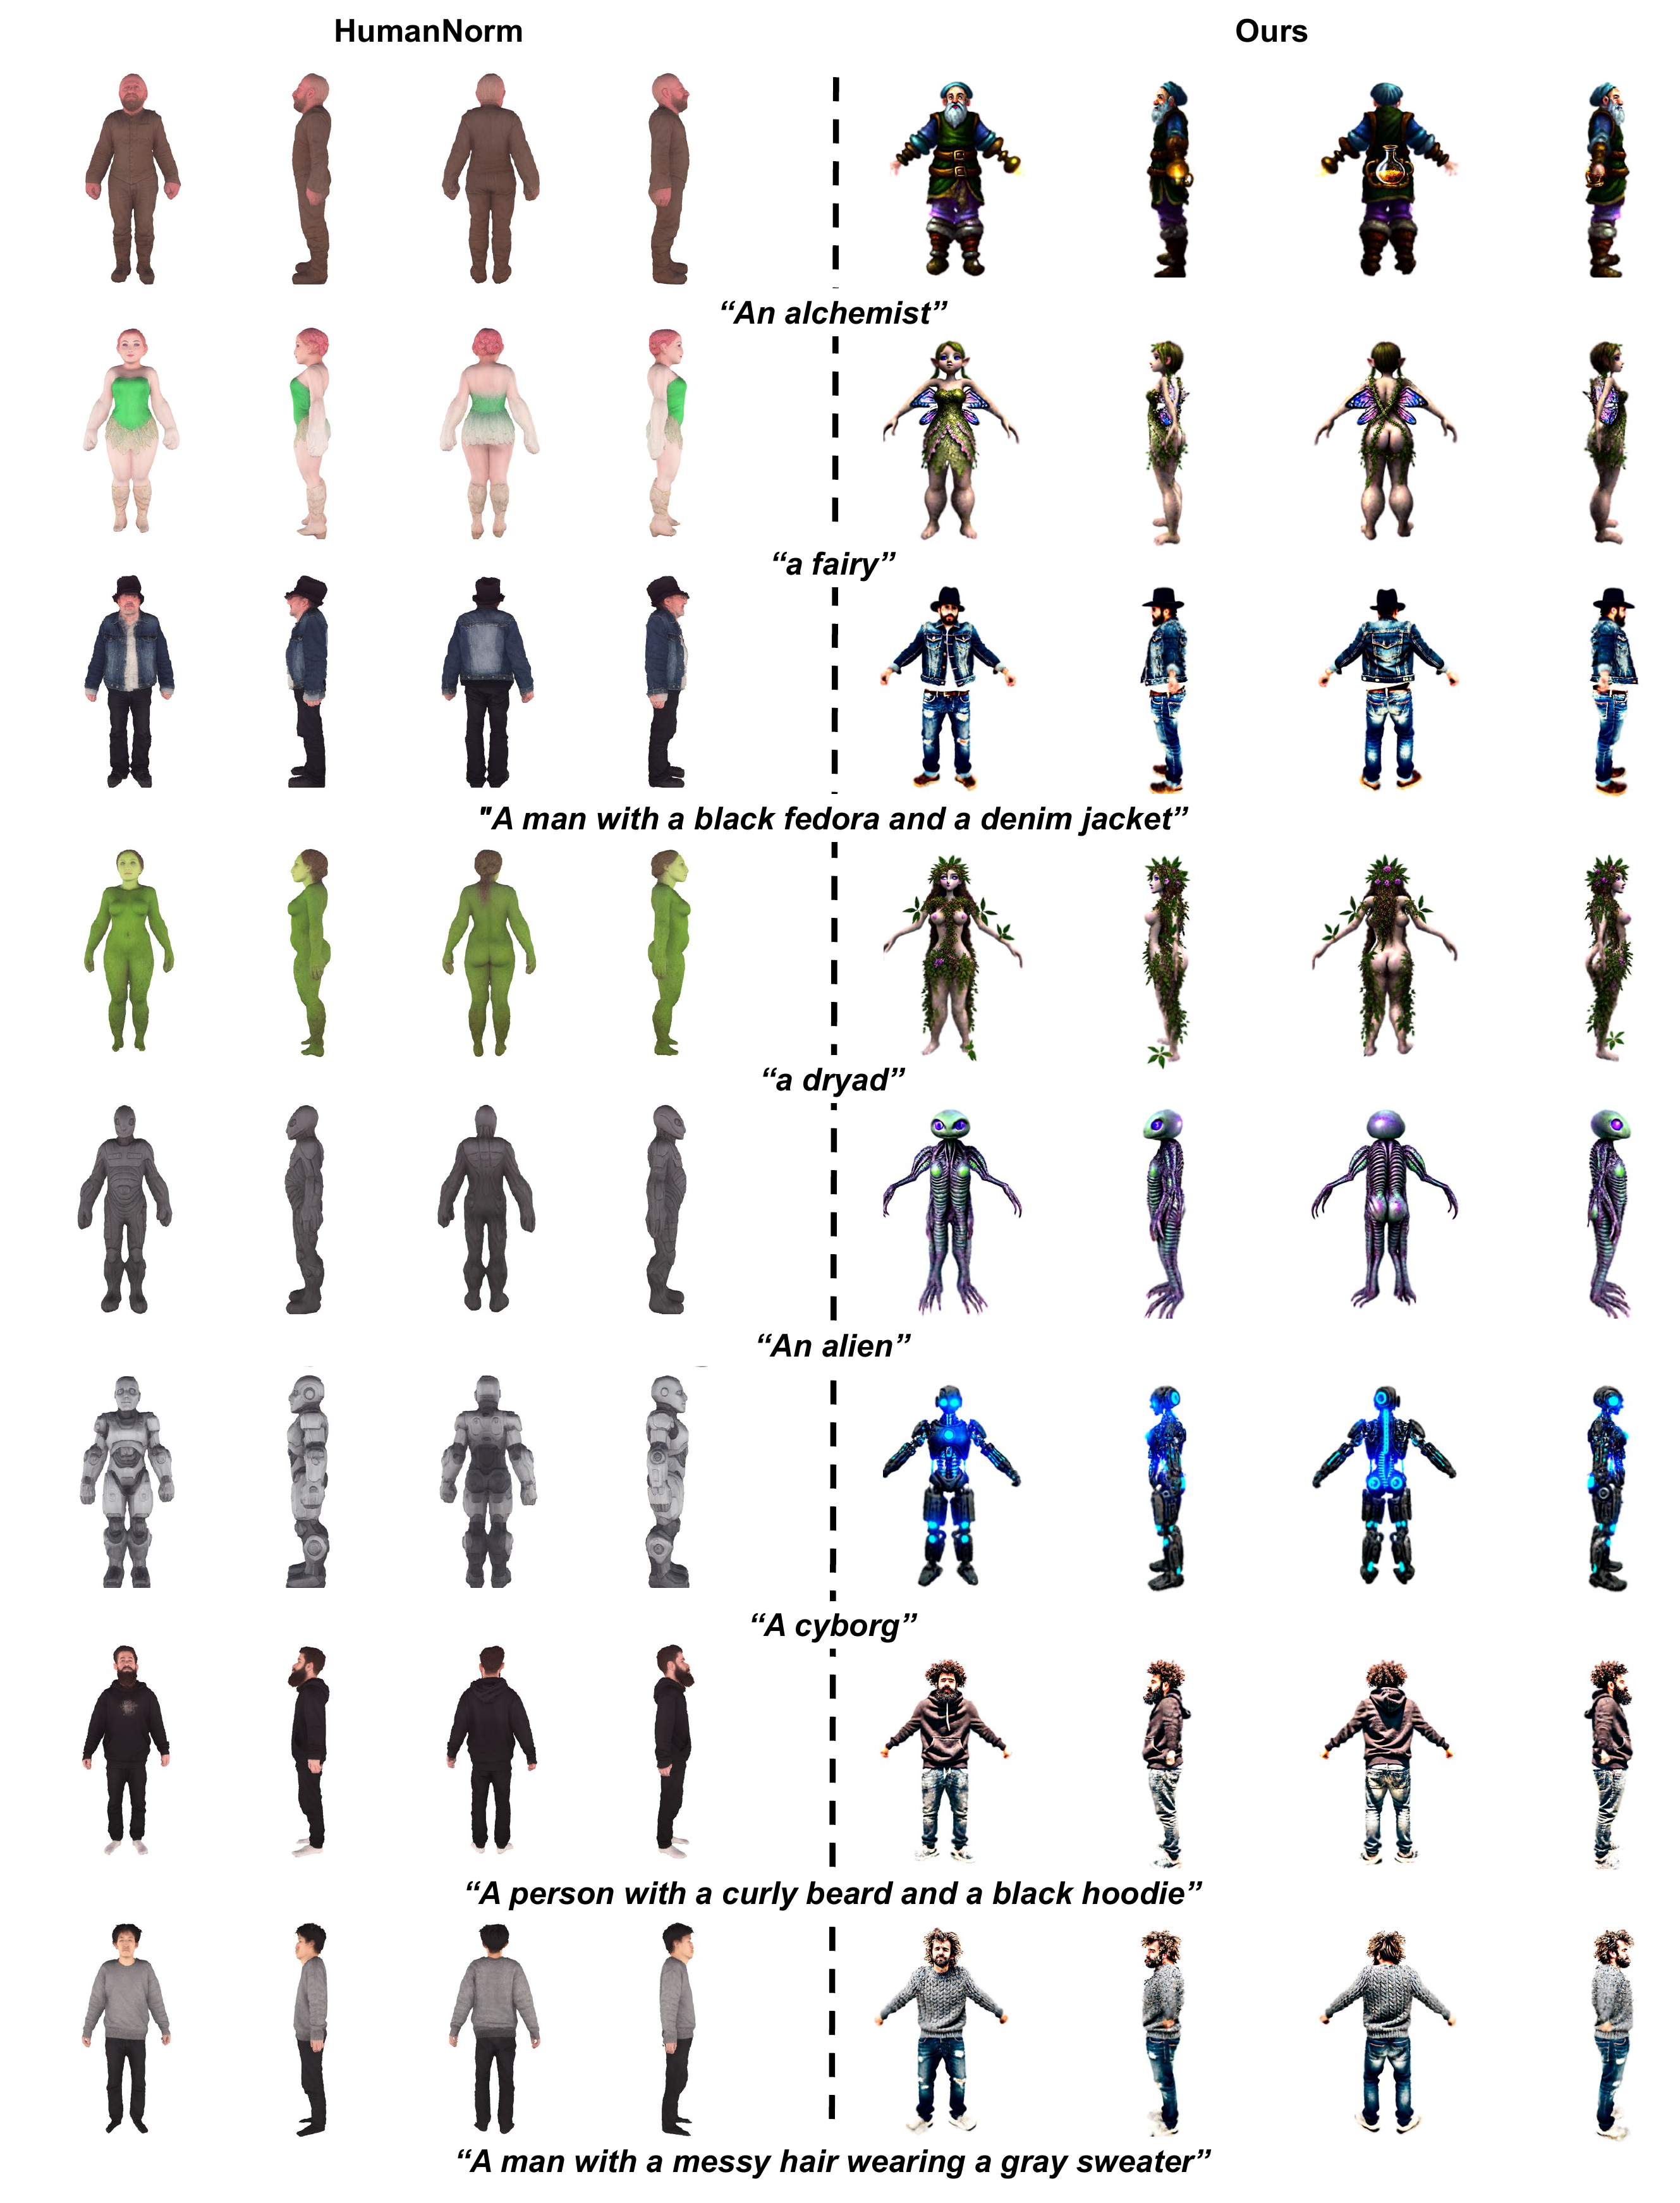} \\
\end{tabular}
\caption{{\bf Qualitative comparison with HumanNorm~\cite{huang2024humannorm}.}
%viewpoints of 0 and 60 degrees,
}
\label{fig:quali_supple_humannorm}
\end{figure*}

\begin{figure*}[t]
\centering
\begin{tabular}{@{}c}
\includegraphics[width=1\linewidth]{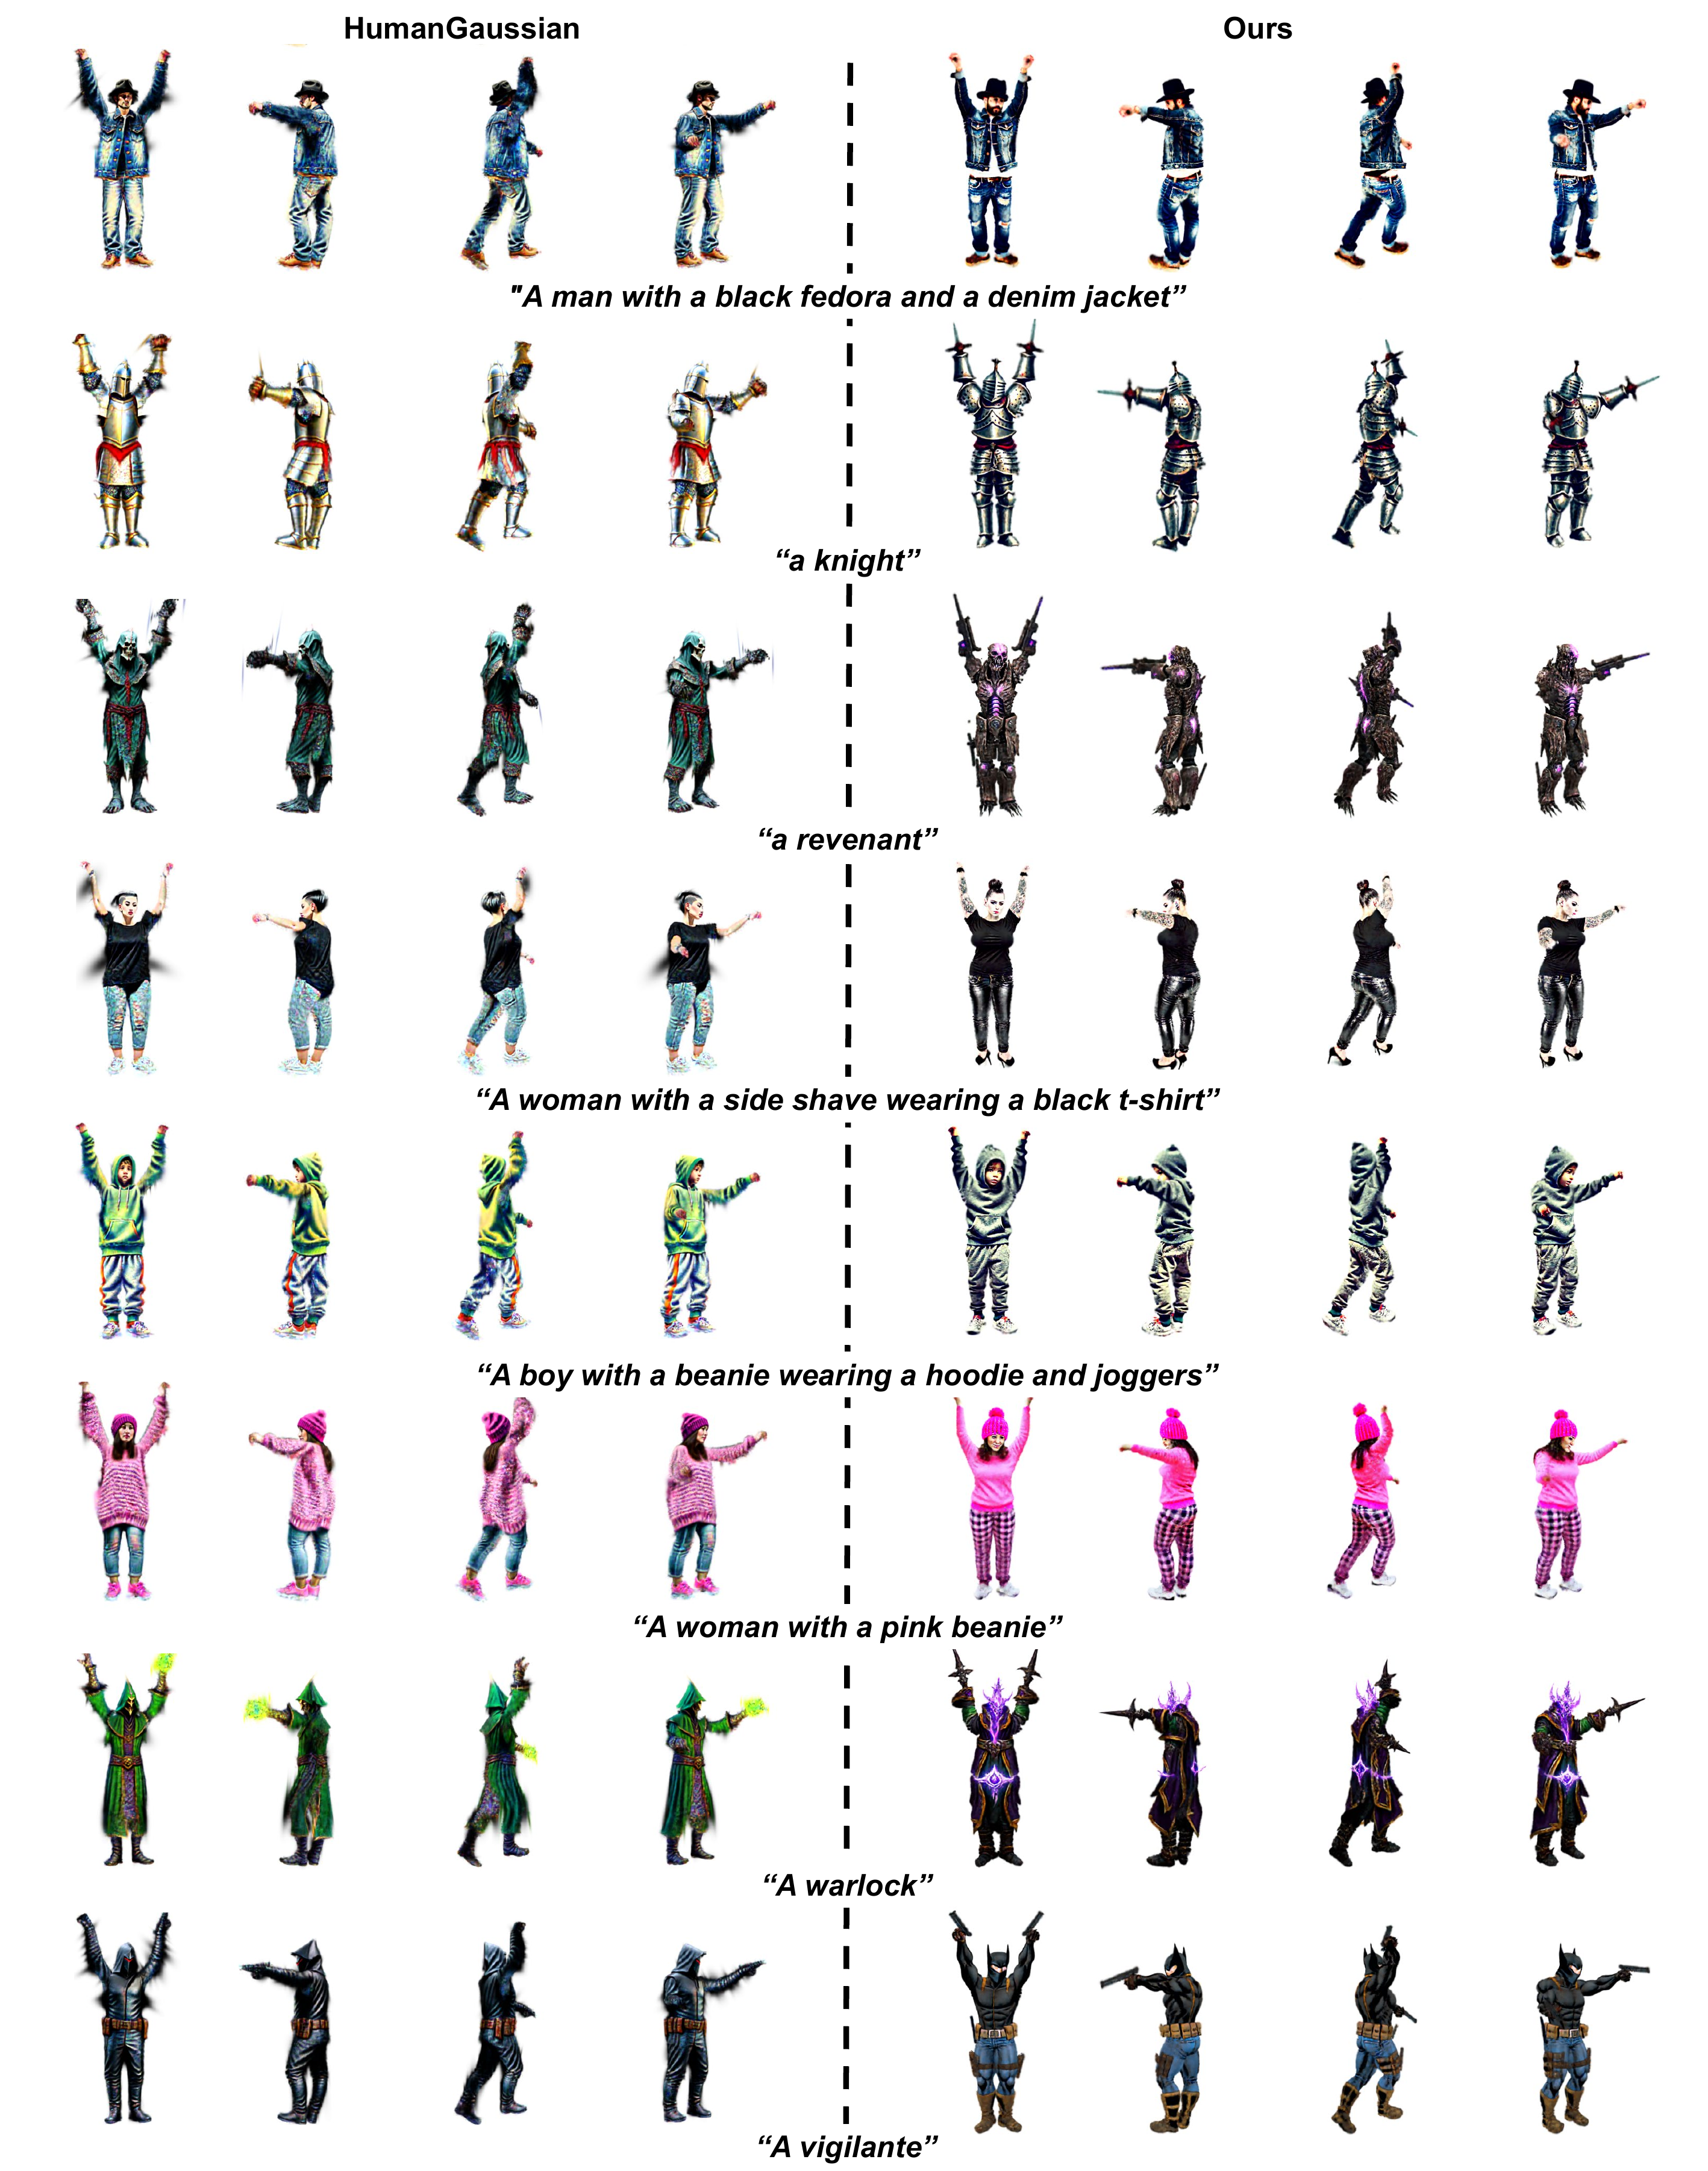} \\
\end{tabular}
\caption{{\bf Qualitative comparison with HumanGaussian~\cite{liu2024humangaussian}.}
%viewpoints of 0 and 60 degrees,
}
\label{fig:quali_supple_humangaussian}
\end{figure*}

\section{Additional Results}
%additional result 티저형식 
In \figref{fig:more_ours}, we present additional examples of avatars generated by our method.
%demonstrating the robustness and generalization performance of the proposed approach.
These examples show the robustness of our approach in handling varying poses and complex body structures while maintaining fine-grained details. Furthermore, the results demonstrate the generalization performance of our method, as it effectively adapts to a wide range of prompts.

\begin{figure*}[t]
\centering
\vspace*{-12\baselineskip}
\begin{tabular}{@{}c}
\includegraphics[width=1\linewidth]{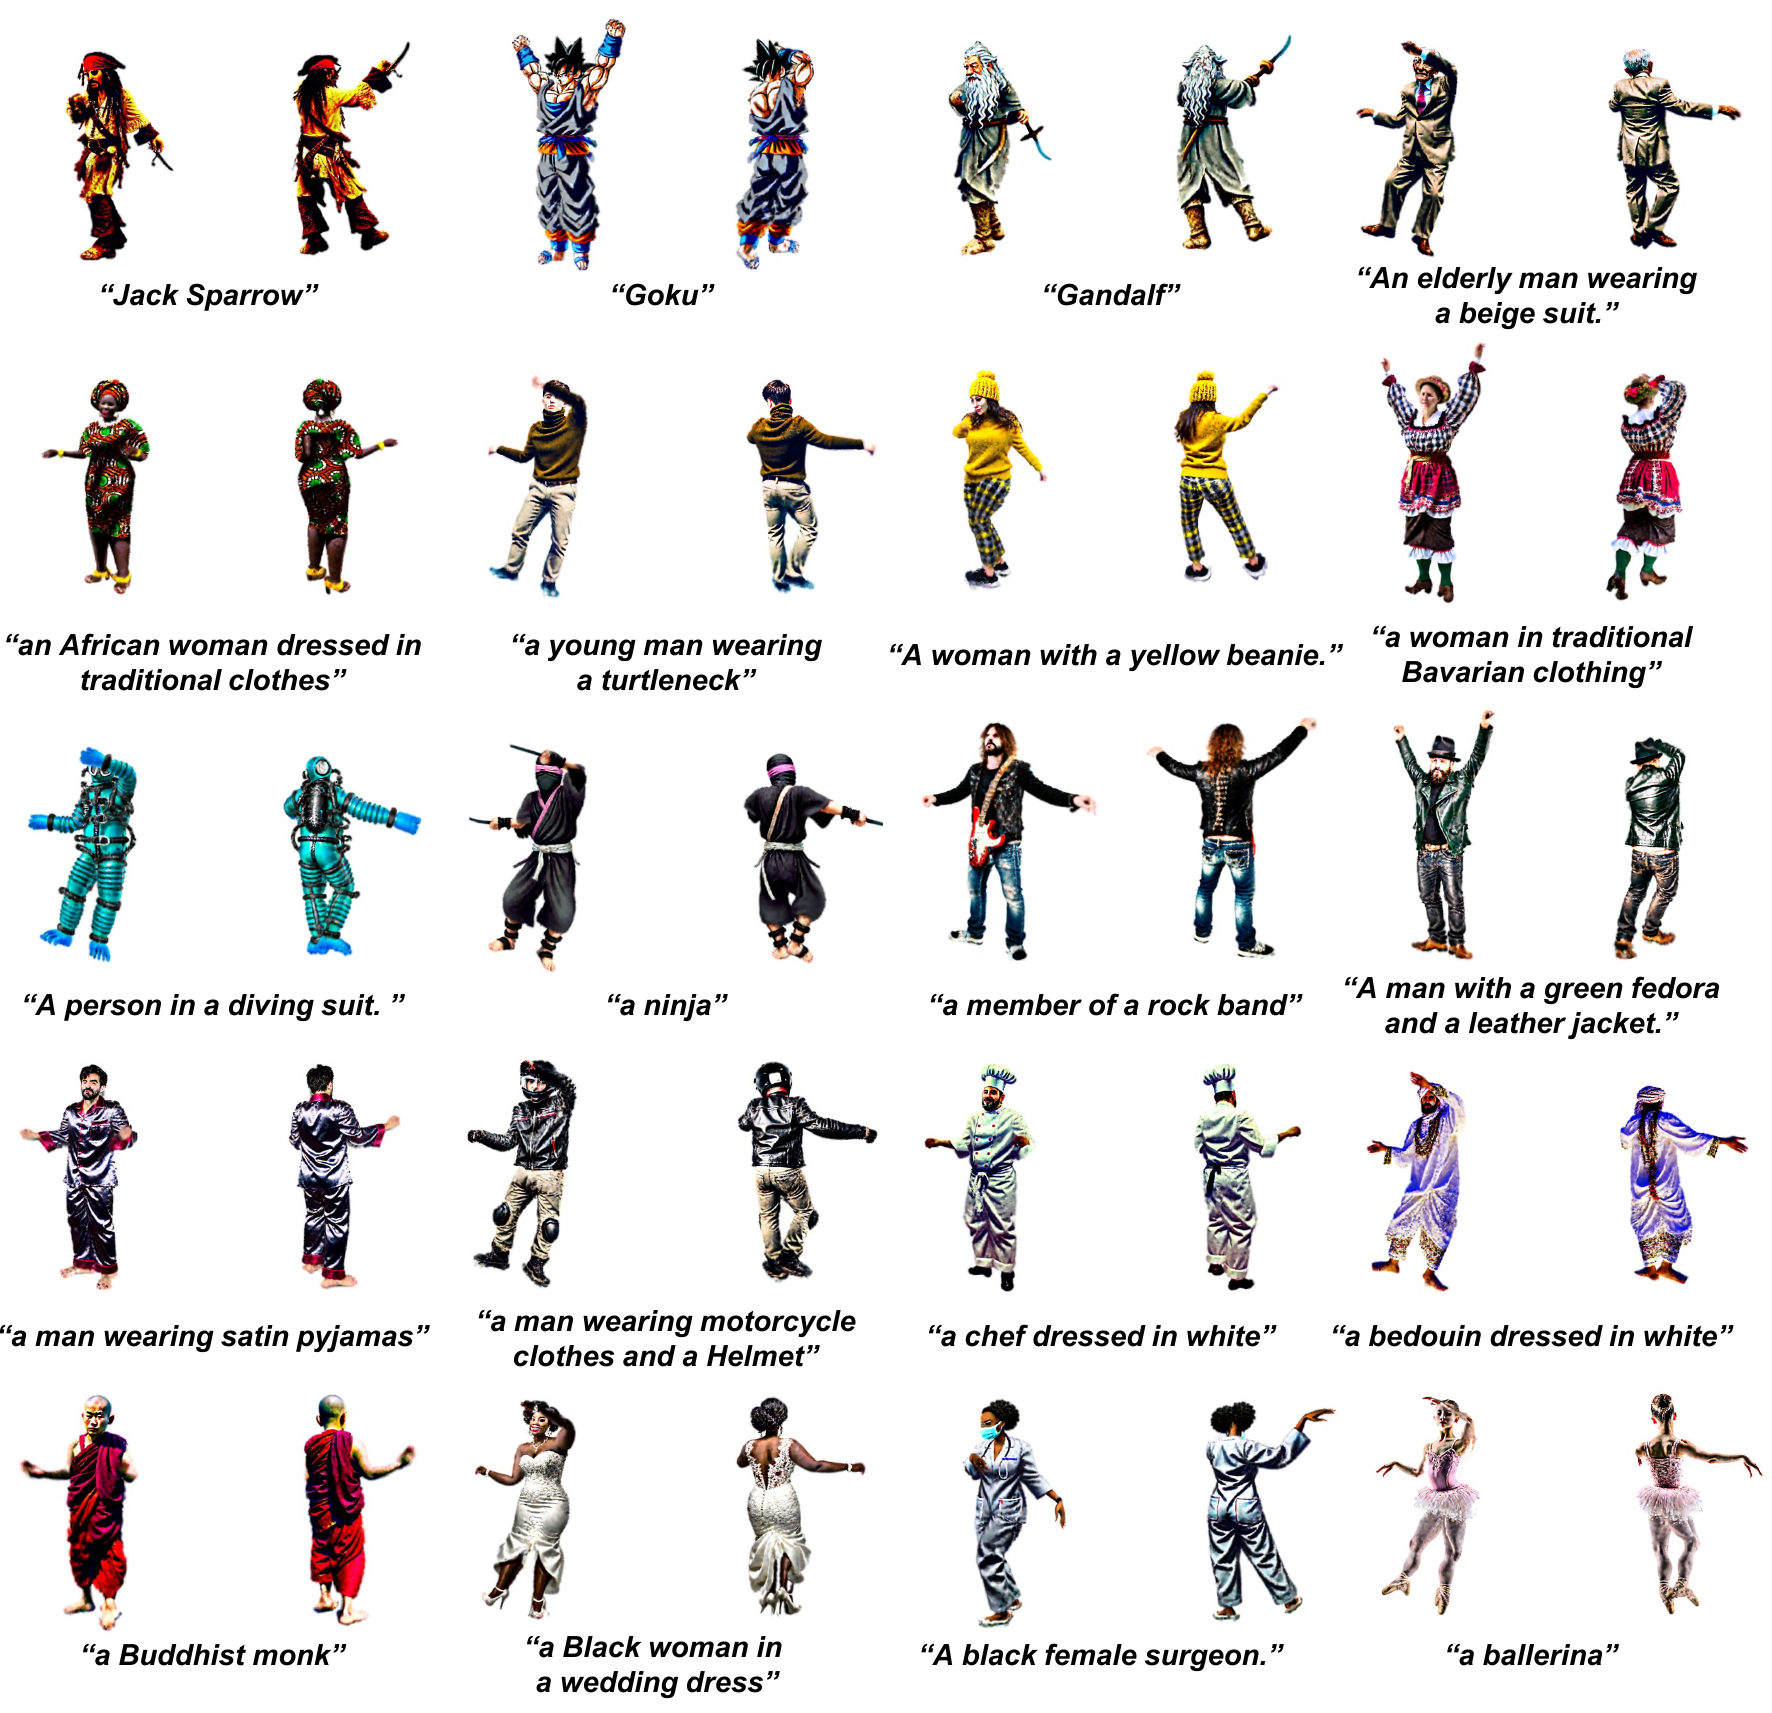} \\
\end{tabular}
\caption{{\bf More examples of 3D human models generated by our method.}
}
\label{fig:more_ours}
\end{figure*}
